# Supplementary material for: Integrating Distributed Energy Resources: Optimal Prosumer Decisions and Impacts of Net Metering Tariffs
Source: arXiv:2204.06115 source file (2022-05-24)
Supplement: Supplementary file 1 [file AppendixA.tex]

This section contains summarizing figures and tables as follows. Fig.\ref{fig:elementsSchematic} presents a schematic summarizing the primary elements that influence BTM DER adoption, which are discussed in depth in section \ref{sec:tariffmodels}. Table \ref{tab:net-basa-comparison} summarizes the generalized two payment models of net metering and feed-in, which are presented in section \ref{subsec:MeteringPolicy}.

\begin{figure*}[htbp]
    \centering
    \includegraphics[scale=0.55]{TariffChart.eps}
    \caption{Elements Affecting BTM DER Adoption (\textcolor{blue}{\small{Should we modify this? or forgo it all-together}}).}
    \label{fig:elementsSchematic}
\end{figure*}

\begin{table*}
\centering
\caption{Summarized comparison between net metering and feed-in.}
\label{tab:net-basa-comparison}
\resizebox{\textwidth}{!}{%
\begin{tabular}{@{}cccccc@{}}
\toprule \toprule
Policy & \begin{tabular}[c]{@{}c@{}}Self \\ consumption\end{tabular} & Meters needed & Billing Period & \begin{tabular}[c]{@{}c@{}}Tariff Model\end{tabular} & Other names \\ \midrule
Net metering & Yes & One & \begin{tabular}[c]{@{}c@{}}Varies from billing cycle \\ to instantaneous\end{tabular} & $P^{\mbox{\tiny NEM}}_\pi(z) =  \pi^{+}z \chi{(z)}+ {\pi}^{-}z (1-\chi{(z)}) +\pi^0$ & \begin{tabular}[c]{@{}c@{}} NEM 1.0, NEM 2.0, full NEM\\ partial NEM, net-billing\\ net purchase and sale, net feed-in\end{tabular} \\
Feed-In & No & Two & Billing cycle & $P_{\pi}^{\mbox{\tiny FiT}}(d,r) =  \pi^+ d - \pi^-  r+\pi^0$ & Buy-all, sell-all, gross feed-in \\ \bottomrule \bottomrule
\end{tabular}%
}
\end{table*}

\begin{table*}[htbp]
\centering
\caption{Summarized literature survey (\textcolor{blue}{\small{Should we modify this? or forgo it all-together}}).}
\label{tab:LiteratureSurvey}
\resizebox{\textwidth}{!}{%
\begin{tabular}{@{}cccccc@{}}
\toprule \toprule
Authors & Addressed issues & Approach & Metering policy & Tariff (rates) & Sell-rate\\ \midrule
    \cite{Tong_DERdynamics:20TAC}        &  Analytical framework for adoption dyanmics    &     Analytical     &         Net metering        &   Two-part  (flat, dynamic)   & Retail-rate           \\
     \cite{CaiRatesImpact:13EP}   &   Utility death spirals    &  Numerical    &  Net metering     &    Two-part (IBR)   &     Retail-rate      \\
      \cite{Next10Report}  &   utility cost recovery and rate-design under higher penetration    &   Numerical   &          Net metering    & Discriminatory two-part        &   Retail-rate and SMC       \\
      \cite{AlvarezConnectionChargesPartII:18TPS}  &    Adoption stability via connection charges  & Analytical     &              Net metering           &    Two-part (flat,dynamic)      &   Retail-rate     \\
      \cite{EID_CostRecoveryShifts:14EP}  &    Cost-recovery and cross-subsidy in net metering   &   Numerical   &           Net metering              &    Two-part (flat)     &   Retail-rate      \\ 
      \cite{BorensteinPrivateNetBenefits:15NBER} & Inequity of IBR under NEM, and skewness of adoption based on income & Numerical & Net metering & One-part  (IBR) &  Retail-rate \\
      \cite{SergiciSubsidiesQuantify:19EJ} & Methodologies for subsidies quantification & Numerical & Net metering & One-part & Retail-rate\\
      \cite{GermeshausenFiT:19ZEW} &Impact of size-based sell-rate differentiation on PV adoption& Numerical & Feed-in & One-part & Size-based\\ 
       \cite{YamamotoPricingEF:12SE} & Social welfare and pricing under feed-in and net metering & Analytical & Feed-in/net metering & Two-part & Varying\\
       \cite{Varaiya_NEMA:19TSG} & Feasibility of community solar under different metering policies & Analytical & Feed-in/net metering & One-part & Varying\\
       \cite{Alahmed_Tong:22IEEETSG} & Prosumer decisions, welfare, cost-shifts and adoption under NEM X & Analytical & Net metering & Two-part & Varying \\
      \bottomrule \bottomrule
\end{tabular}%
}
\end{table*}
